# Supplementary material for: Explicit Diversity Conditions for Effective Question Answer Generation with Large Language Models
Source: arXiv:2406.17990 source file (2024-06-26)
Supplement: Supplementary file 1 [file Appendix.tex]

\section{Appendix}

\subsection{Context based binary classification}
\label{MultiRC_res}
To evaluate PAG-LLM on context based binary classification tasks, we experimented with MultiRC \cite{khashabi2018looking} where multiple candidate answers can be correct for a given question based on a passage. We concatenate passage, question and candidate answer and IFT LLaMa to predict whether the candidate answer is correct or not. Similar to our observations in \cref{ID_result_table}, PAG-LLM achieves 87.1\%F1 score compared to 85.8\% F1 score of baseline LLaMa.

Prompt example: Given this question: "what is the day off request status", Select the best answer from the following candidates:
\begin{itemize}
\item pred: request\_status, conf: 0.28
\item pred: pto\_request\_status, conf: 0.98
\item pred: pto\_request\_status, conf: 0.86
\item pred: pto\_request\_status, conf: 0.98
\item pred: pto\_request\_status, conf: 0.98
\item pred: pto\_request\_status, conf: 0.98
\end{itemize}

\subsection{Examples}
The table \cref{Examplefig} shows examples of misclassification and out-of-vocabulary corrections from our PAG-LLM approach. 

\begin{table*}[t]
   \centering
   \small
    \begin{tabular}{rlll}
     \hline
     & Input & Prediction & Confidence\\ \hline
     Original: & what is the day off request status & request\_status & \textcolor{red}{0.28}\\
     Paraphrase 1:& Can you provide me with the status of my day off request? & pto\_request\_status & \textcolor{teal}{0.98}\\
     Paraphrase 2:& How is my day off request doing? & pto\_request\_status & \textcolor{red}{0.86}\\
     Paraphrase 3:& What is the current status of my day off request? & pto\_request\_status & \textcolor{teal}{0.98}\\
     Paraphrase 4:& Could you let me know the status of my day off request? & pto\_request\_status & \textcolor{teal}{0.98}\\
     Paraphrase 5:& What is the update on my day off request status? & pto\_request\_status & \textcolor{teal}{0.98}\\
     \hline
     \multicolumn{2}{r}{Final Prediction: pto\_request\_status {Aggregation EXAMPLE}}&
     \multicolumn{2}{r}{Gold Label: pto\_request\_status} \\
     \hline
     Original: & what is the reason humans even exist & explain\_meaning\_of\_life & \textcolor{red}{0.11}\\
     Paraphrase 1:& What is the purpose of human existence? & meaning\_of\_life & \textcolor{teal}{0.32}\\
     Paraphrase 2:& Why do humans exist in the world? & The meaning of life & \textcolor{red}{0.05}\\
     Paraphrase 3:& What is the cause of human existence? & $NULL$ & \textcolor{red}{0.07}\\
     Paraphrase 4:& What is the explanation for the existence of humans? & explain\_life & \textcolor{red}{0.21}\\
     Paraphrase 5:& What is the rationale behind the existence of human beings? & rational\_existence & \textcolor{red}{0.08}\\
     \hline
     \multicolumn{2}{r}{Final Prediction: meaning\_of\_life \textcolor{red}{Aggregation EXAMPLE}} &
     \multicolumn{2}{r}{Gold Label: meaning\_of\_life} \\
     \hline
   \end{tabular}
   
   \caption{\small \label{Exampletable}Examples from CLINC, where LLM classifies incorrect label (1st example) and out-of-vocabulory (OOV) class label (2nd example). In the 1st example, paraphrases generated by PAG-LLM enables correct classification decisions with high confidence scores. Thus, even simple majority voting aggregation leads to the correct class prediction. In the 2nd example, only paraphrase2 from PAG-LLM enables correct classification while remaining paraphrases and the original query have OOV class labels. PAG-LLM aggregates texts of input, paraphrases, their labels and confidences to finally predict the correct class label.}
   \vspace{-5mm}
\end{table*}

\begin{figure}%[t!] % [width=2\columnwidth, height=180pt]
\includegraphics[width=2\columnwidth]{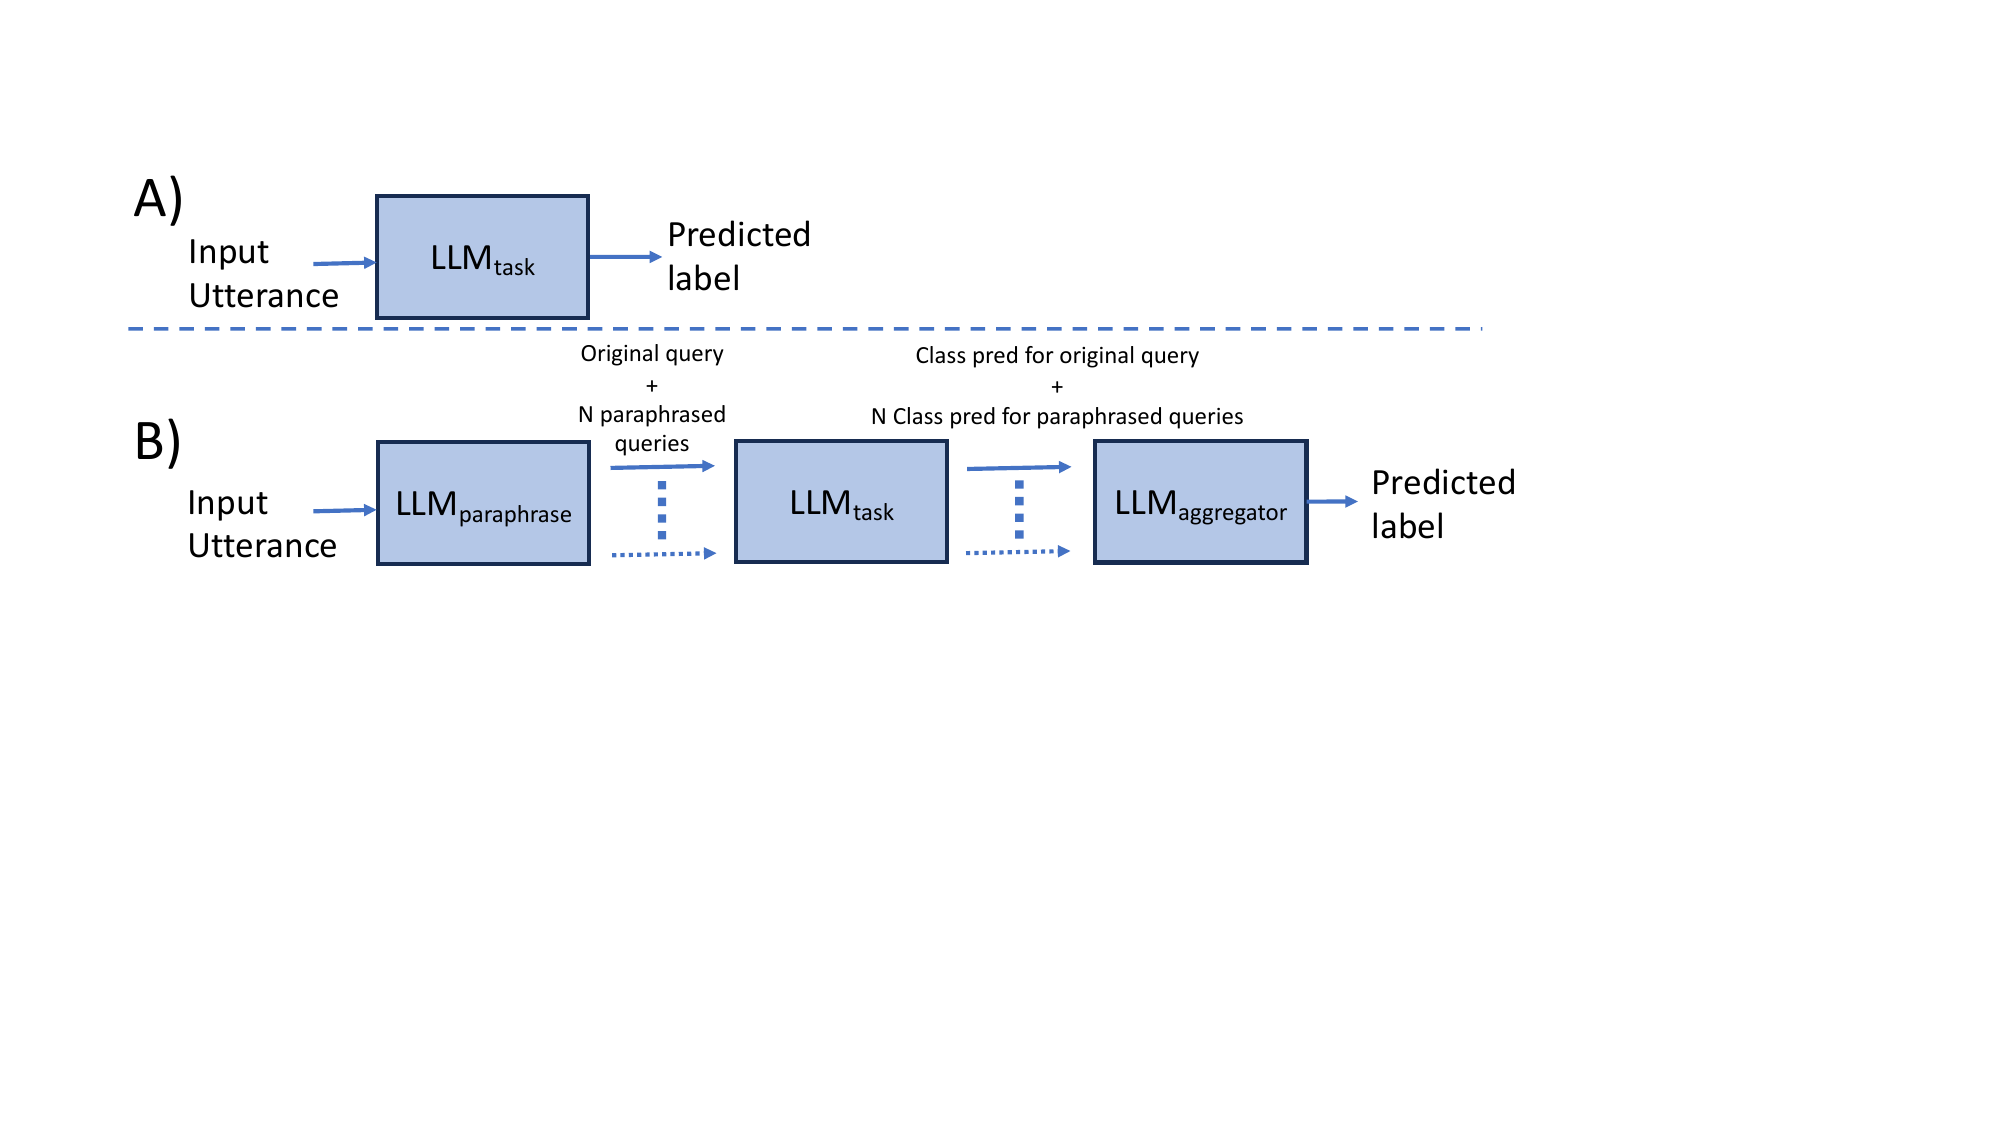} 
 \caption{\footnotesize Figure depicting the process of PAG-LLM. %\textcolor{red}{A) The top part is similar to baseline LLM where prediction is considered as the final label if confidence is high. This corresponds to roughly 90.2\% of the inference data (discussed in \cref{InferenceCost}).} B) 
 The top part shows the first step where LLM classifies the original query. Only if the classification confidence is low (i.e., 32\% of the inference data in CLINC (\cref{Analysis}), original query is given to the LLM for generating paraphrases which are then given to LLM for classification. Finally, LLM aggregates the predicted class labels from paraphrases and the original query.   }
  \label{fig:ExampleblockDiag}
  \vspace{-5mm}
\end{figure}
